# Supplementary material for: The dog-and-rabbit chase problem
Source: arXiv:2206.02745 source file (2022-06-06)
Supplement: Supplementary file 1 [file pdfa-supp.tex]

\pdfcompresslevel=0
%\pdfmapfile{+cmsy-v2.map}

%***************************
% generate ToUnicode entries
%___________________________
% \input glyphtounicode.tex
% \input glyphtounicode-cmr.tex
% \pdfgentounicode=1

%***************************************************************************
% \convertDate converts D:20080419103507+02'00' to 2008-04-19T10:35:07+02:00
%___________________________________________________________________________
\def\convertDate{%
    \getYear
}

{\catcode`\D=12
 \gdef\getYear D:#1#2#3#4{\edef\xYear{#1#2#3#4}\getMonth}
}
\def\getMonth#1#2{\edef\xMonth{#1#2}\getDay}
\def\getDay#1#2{\edef\xDay{#1#2}\getHour}
\def\getHour#1#2{\edef\xHour{#1#2}\getMin}
\def\getMin#1#2{\edef\xMin{#1#2}\getSec}
\def\getSec#1#2{\edef\xSec{#1#2}\getTZh}
\def\getTZh +#1#2{\edef\xTZh{#1#2}\getTZm}
\def\getTZm '#1#2'{%
    \edef\xTZm{#1#2}%
    \edef\convDate{\xYear-\xMonth-\xDay T\xHour:\xMin:\xSec+\xTZh:\xTZm}%
}

\expandafter\convertDate\pdfcreationdate 

%**************************
% get pdftex version string
%__________________________
\newcount\countA
\countA=\pdftexversion
\advance \countA by -100
\def\pdftexVersionStr{pdfTeX-1.\the\countA.\pdftexrevision}

%*********
% XMP data
%_________
% \usepackage{xmpincl}
% \includexmp{pdfa-1b}

%********
% pdfInfo
%________
\pdfinfo{%
/Title(\Title)
/Author(\Author)
/Subject(\Subject)
/Keywords(\Keywords)
/ModDate(\pdfcreationdate)
/Trapped/False
/RJP.Copyright(Romanian Academy Publishing House (c) \xYear)
}

%*************************
% explicit interword space
%_________________________

\expandafter\ifx\csname pdfgeninterwordspace\endcsname\relax
    \message{\string\pdfgeninterwordspace\space not supported by this version of pdftex}
\else
    \pdfmapline{+dummy-space <dummy-space.pfb}
    \pdfgeninterwordspace=1
\fi
